# Supplementary material for: Symmetry Breaking of the Persistent Spin Helix in Quantum Transport
Source: arXiv:1801.05657 ancillary file (2018-01-17)
Supplement: Supplementary file 1 [file SOM.pdf]

Supplementary Information

# Symmetry Breaking of the Persistent Spin Helix in Quantum Transport

Pirmin J. Weigele,[1,*] D. C. Marinescu,[2,*] Florian Dettwiler,[1] Jiyong Fu,[3] Shawn Mack,[4] J. Carlos Egues,[5] David D. Awschalom,[6] and Dominik M. Zumbühl[1]

[1]*Department of Physics, University of Basel, CH-4056, Basel, Switzerland*

[2]*Department of Physics and Astronomy, Clemson University, Clemson, South Carolina 29634, USA*

[3]*Instituto de Física, Universidade de Brasília, Brasília-DF 70919-970, Brazil*

[4]*Naval Research Laboratory, Washington, DC 20375, USA*

[5]*Instituto de Física de São Carlos, Universidade de São Paulo, 13560-970 São Carlos, São Paulo, Brazil*

[6]*Institute for Molecular Engineering, University of Chicago, Chicago, Illinois 60637, USA*

[*] These authors contributed equally to this work.

## CONTENTS


I. Calculation of the Quantum Corrections 1

A. Quantum Corrections in Presence of a Magnetic Field 4

II. Full Account of Data 9

A. Summary of extracted data 10

III. Details on evaluating $B_{SO-}$ and $B_{SO3}$ 18

A. Symmetry point determination and value of $B_{SO3}$ 18

B. Validity of the theory 18

References 21


## I. CALCULATION OF THE QUANTUM CORRECTIONS

The quantum corrections to the conductivity are obtained by considering that the electron states used in calculating the scattering matrix element that determines the relaxation rate are themselves modified by previous scattering processes. The coherent superposition of the (time-reversed) scattered states leads to stable transport modes associated with a decrease in the conductivity value known as the localization correction. Next we outline the main steps in the calculation of these quantum corrections to the conductivity. We follow closely the works of Iordanskii et al. [1], Knap et al. [2] and Marinescu [3]

In the following, we assume that scattering on impurities is elastic, spin-independent, and involves only states at the Fermi surface, whose density of states per spin is $\nu_0 = m^*/2\pi\hbar^2$. The scattering matrix element $V_{\mathbf{p},\mathbf{p}'}$ of two electrons with momenta $\mathbf{p}$ and $\mathbf{p}'$, dependent only of the angle $\varphi$ between the incident and scattered directions, gives rise to a scattering lifetime $\tau_0$

$$\frac{\hbar}{\tau_0} = \nu_0 \int |V_{\mathbf{p},\mathbf{p}'}|^2(\varphi) d\varphi \;, \tag{S1}$$

within the first Born approximation. The propagation of the particles is described by impurity averaged advanced (A) and retarded (R) Green's functions, written in terms of the

single particle Hamiltonian, $H_{\mathbf{p}}$ (see Eq. (2) in the main text) as,

$$G^{\pm}(\mathbf{p},\epsilon)=\frac{1}{\epsilon-H_{\mathbf{p}}\pm i\frac{\hbar}{2\tau_0}}. \tag{S2}$$

As discussed in the main text, the main object in the theory of localization is the Cooperon operator, which represents an impurity averaged scattering amplitude for an electron state $\mathbf{p}$ that is almost perfectly backscattered into $\mathbf{p}'\approx-\mathbf{p}$; $\hbar\mathbf{q}=\mathbf{p}+\mathbf{p}'$, $\hbar q\ll p$ denotes deviations from the $\mathbf{p}'=-\mathbf{p}$ case. In this limit, the quantum corrections to the conductivity can be determined in terms of the Cooperon eigenvalues $C_i(\mathbf{q})$ [4, 5]

$$\Delta\sigma=-\frac{2e^2D\tau_0^2\nu_0}{\hbar^2}\sum_{\mathbf{q},i}C_i(\mathbf{q})\ , \tag{S3}$$

where $D=v_F^2\tau_1/2$ is the 2D diffusion coefficient, $i$ indexes the singlet and triplet spin states (to be discussed further below), $v_F$ the Fermi velocity and $\tau_1$ the transport scattering time. The anisotropy of the scattering matrix element $V_{\mathbf{p},\mathbf{p}'}$ [6] results in a series of transport times, of which $\tau_1$ is the first ($n=1$), defined by

$$\frac{\hbar}{\tau_n}=\nu_0\int|V_{\mathbf{p},\mathbf{p}'}|^2(1-\cos n\varphi)d\varphi\ , \tag{S4}$$

with $n=1,2,3...$ The impurity mediated Cooperon equation is

$$C_{\mathbf{p},\mathbf{p}'}(\mathbf{q})=|V_{\mathbf{p},\mathbf{p}'}|^2+\sum_{\mathbf{p}''}|V_{\mathbf{p},\mathbf{p}''}|^2G^{+}_{-\mathbf{p}''+\hbar\mathbf{q},\epsilon+\hbar\omega}G^{-}_{\mathbf{p}'',\epsilon}C_{\mathbf{p}'',\mathbf{p}'}\ . \tag{S5}$$

To proceed, we first integrate the kernel in Eq. (S5) over the kinetic energy $p^2/2m^*$ in the complex plane then expand the result in terms of the scattering rate $\hbar/\tau_0$, the leading term in the denominator. Since after many scattering events the spin directions of the two electron spins traveling along time-reversed paths are completely uncorrelated, we label them by distinct indices $\sigma$ and $\rho$, respectively. Thus Eq. (S5) becomes,

$$\begin{aligned}C_{\mathbf{p},\mathbf{p}'}(\mathbf{q})=|V_{\mathbf{p},\mathbf{p}''}|^2+\nu_0\int_0^{2\pi}d\varphi_{\mathbf{p}''}|V(\varphi_p-\varphi_{p''})|^2\left\{1+i\omega\tau_0+i\mathbf{q}\cdot\mathbf{v}_{\mathbf{p}''}\tau_0-(i\mathbf{q}\cdot\mathbf{v}_{\mathbf{p}''})^2\tau_0^2\right.\\+\left[i\mathbf{\Omega}_{\mathbf{p}''}\times(\sigma+\rho)\cdot\hat{y}\right]\tau_0-\left[i\mathbf{\Omega}_{\mathbf{p}''}\times(\sigma+\rho)\cdot\hat{y}\right]^2\tau_0^2\\\left.-\,2\left(\mathbf{q}\cdot\mathbf{v}_{\mathbf{p}''}\right)\left[\mathbf{\Omega}_{\mathbf{p}''}\times(\sigma+\rho)\cdot\hat{y}\right]\tau_0^2\right\}C_{\mathbf{p}'',\mathbf{p}'}.\end{aligned} \tag{S6}$$

Let us now search for an iterative solution by expanding the Cooperon in terms of harmonics: $C_{\mathbf{p},\mathbf{p}'}(q) = C^{(0)}_{\mathbf{p},\mathbf{p}'}(q) + C^{(1)}_{\mathbf{p},\mathbf{p}'}(q)\cos\varphi_{\mathbf{p}} + C^{(2)}_{\mathbf{p},\mathbf{p}'}(q)\cos 2\varphi_{\mathbf{p}} + \ldots$, with $\varphi_p$ being the angle between $\hbar\mathbf{q} = \mathbf{p} + \mathbf{p}'$ and $\mathbf{p}$. The first order correction $C^{(1)}_{\mathbf{p},\mathbf{p}'}(q)$ is readily written in terms of the components of total spin $\mathbf{J} = (\sigma + \rho)/2$ (in $\hbar$ units) of the two electrons

$$\begin{aligned} &\int_0^{2\pi} d\varphi_{\mathbf{p}''} |V(\varphi_{\mathbf{p}} - \varphi_{\mathbf{p}''})|^2 \{vq\cos\varphi_{p''} \\ &+ 2\left[(\alpha - \beta)\sin\varphi_{\mathbf{p}''} - \beta_3 \sin 3\varphi_{\mathbf{p}''}\right] J_x \\ &- 2\left[(\alpha + \beta)\cos\varphi_{\mathbf{p}''} - \beta_3 \cos 3\varphi_{\mathbf{p}''}\right] J_z\} \ . \end{aligned} \tag{S7}$$

Here $\varphi_{\mathbf{p}''}$ is the angle between $\mathbf{p}''$ and $\mathbf{q}$, i.e., the same angular dependence of $C_{\mathbf{p}'',\mathbf{p}'}(\mathbf{q})$. Noticing that

$$\begin{aligned} &\nu_0 \int_0^{2\pi} d\varphi_{\mathbf{p}''} |V(\varphi_{\mathbf{p}} - \varphi_{\mathbf{p}''})|^2 \cos n\varphi_{\mathbf{p}''} \\ &= \nu_0 \int_0^{2\pi} d\varphi |V(\varphi_{\mathbf{p}} - \varphi_{\mathbf{p}''})|^2 \cos n(\varphi_{\mathbf{p}} - \varphi_{\mathbf{p}''}) \cos n\varphi_{\mathbf{p}} \\ &= \cos n\varphi_{\mathbf{p}} \left(\frac{1}{\tau_0} - \frac{1}{\tau_n}\right) \\ &= \frac{(\tau_n - \tau_0)}{\tau_0 \tau_n} \cos n\varphi_{\mathbf{p}} \approx \frac{(\tau_n - \tau_0)}{\tau_0^2} \cos n\varphi_{\mathbf{p}} \end{aligned} \tag{S8}$$

with $\tau_1$ and $\tau_3$ given by Eq. (S4), we can cast the first-order correction to the Cooperon in the form

$$\begin{aligned} C^{(1)} &= i(\tau_1 - \tau_0)\left[\mathbf{v}_{\mathbf{p}''} \cdot \mathbf{q} + 2(\alpha - \beta) J_x \sin\varphi_{\mathbf{p}''} \right. \\ &\left. - 2(\alpha + \beta) J_z \cos\varphi_{\mathbf{p}''}\right] \\ &- i(\tau_3 - \tau_0)\left(-2\beta_3 J_x \sin 3\varphi_{\mathbf{p}''} + 2\beta_3 J_z \cos 3\varphi_{\mathbf{p}''}\right) C^{(0)} \ . \end{aligned} \tag{S9}$$

Upon inserting $C = C^{(0)} + C^{(1)}$ in the kernel of Eq. (S5) and performing some simplifications, all contributions proportional to $\tau_0$ drop out. A further linearization of Eq. (S5) yields the lowest order expression the for zeroth-order harmonic of the Cooperon

$$C^{(0)}_{\mathbf{p},\mathbf{p}'}(\mathbf{q}) = \frac{|V_{\mathbf{p},\mathbf{p}'}|^2}{\tau_0 \mathcal{H}} \ , \tag{S10}$$

where $\mathcal{H}$ is an operator in the 4-dimensional space associated with the total angular momentum $J$, corresponding to the addition of the two spins, reading

$$\begin{aligned}\mathcal{H} = Dq^2 + \frac{1}{\tau_\varphi} + 2k_F^2\left[(\alpha+\beta)^2\tau_1 + \beta_3^2\tau_3\right]J_z^2 \\ + 2k_F^2\left[(\alpha-\beta)^2\tau_1 + \beta_3^2\tau_3\right]J_x^2 \\ + 2k_F(\alpha-\beta)\tau_1 v q_z J_x - 2k_F(\alpha+\beta)\tau_1 v q_x J_z \ . \end{aligned} \tag{S11}$$

where we have replaced $-i\omega$ by $1/\tau_\varphi$, the dephasing time, a descriptor of the inelasticity of the propagation. For convenience we introduce the following parameters

$$\begin{aligned} Q_\pm &= \frac{2m^*(\alpha\pm\beta)}{\hbar^2} \ , \\ Q_3 &= \frac{2m^*\beta_3}{\hbar^2}\sqrt{\frac{\tau_3}{\tau_1}} \ . \end{aligned} \tag{S12}$$

We can then recast $\mathcal{H}$ as

$$\begin{aligned}\mathcal{H} = Dq^2 + \frac{1}{\tau_\varphi} + D\left\{\left[Q_+^2 + Q_3^2\right]J_z^2 + \left[Q_-^2 + Q_3^2\right]J_x^2 \right. \\ \left. + 2Q_- q_z J_x - 2Q_+ q_x J_z\right\} \ . \end{aligned} \tag{S13}$$

At this point we can diagonalize $\mathcal{H}$ and easily find eigenvalues $C_i(\mathbf{q})$ of the Cooperon operator (via Eq. S10) and from Eq. S3 determine the weak localization corrections [1]. In the next section we generalize the above procedure by including a magnetic field, essential for probing weak localization experimentally, and outline the derivation of the general weak-localization formula first derived in this work (see Eq. (5) in the main text).

### A. Quantum Corrections in Presence of a Magnetic Field

In the presence of a quantizing magnetic field, the position representation of the Green's function $G^\pm(\mathbf{r},\mathbf{r}')$ is modified as [7]

$$\tilde{G}^\pm(\mathbf{r},\mathbf{r}') = e^{\frac{ie}{\hbar}\int_{\mathbf{r}}^{\mathbf{r}'}\mathbf{A}(\mathbf{l})\cdot d\mathbf{l}}G^\pm(\mathbf{r},\mathbf{r}') \ , \tag{S14}$$

a good approximation when the Landau orbit is larger than the Fermi wavelength. Because of this approximation for the Green's functions, it is convenient to work in position repre-

sentation. By following essentially the same protocol as in the previous section, i.e., from Eqs. (S5) to (S10), but now in the position representation, we find that the denominator of the zeroth-order Cooperon acquires a phase (i.e., $\mathcal{H} \to \tilde{\mathcal{H}}$ in Eq. S10)

$$\tilde{\mathcal{H}}(\mathbf{r}, \mathbf{r}') = e^{i\frac{2e}{\hbar}\int_{\mathbf{r}}^{\mathbf{r}'} \mathbf{A}(\mathbf{l})\cdot d\mathbf{l}} \mathcal{H}(\mathbf{r}, \mathbf{r}') \ , \tag{S15}$$

where the Fourier transform of $\mathcal{H}$ in the absence of the magnetic field is given in Eq. (S13). This approximation is correct for $|\mathbf{r} - \mathbf{r}'| \ll l$, where $l$ is the mean free path. In this case, the integral defining the phase in Eq. S15 can be linearized to $\mathbf{A} \cdot (\mathbf{r}' - \mathbf{r})$. Now we can solve the generalized eigenfunction-eigenvalue equation for $\mathcal{H}(\mathbf{r}, \mathbf{r}')$,

$$\int e^{i\frac{2e}{\hbar}\mathbf{A}\cdot(\mathbf{r}'-\mathbf{r})} \mathcal{H}(\mathbf{r}, \mathbf{r}')\psi(\mathbf{r}')d\mathbf{r}' = \mathcal{E}\psi(\mathbf{r}) \ , \tag{S16}$$

by taking advantage that the difference $\Delta\mathbf{r} = \mathbf{r}' - \mathbf{r}$ is small so that the integrand above can be expanded as a power series of $\Delta\mathbf{r}$. The kernel of the integral equation becomes,

$$\begin{aligned}
&\mathcal{H}(\mathbf{r}' - \mathbf{r}) \left[1 + i\frac{2e}{\hbar}\mathbf{A}\cdot\Delta\mathbf{r} + \frac{1}{2}\left(i\frac{2e}{\hbar}\mathbf{A}\cdot\Delta\mathbf{r}\right)^2\right] \\
&\times \left[\psi(\mathbf{r}) + \nabla\psi\cdot\Delta\mathbf{r} + \frac{1}{2}(\nabla\psi\cdot\mathbf{A})\right] \\
&= \mathcal{H}(\mathbf{r}' - \mathbf{r}) \left\{1 + \left(\nabla + i\frac{2e}{\hbar}\mathbf{A}\right)\cdot\Delta\mathbf{r} \right. \\
&\left. + \frac{1}{2}\left[\left(\nabla + i\frac{2e}{\hbar}\mathbf{A}\right)\cdot\Delta\mathbf{r}\right]^2\right\}\psi(\mathbf{r}) \ .
\end{aligned} \tag{S17}$$

By using the identity

$$\int d\mathbf{r}'\mathcal{H}(\mathbf{r}' - \mathbf{r})\,(\Delta\mathbf{r})^n = \frac{\partial^n \mathcal{H}(\mathbf{q})}{i^n \partial q^n}\,|_{\mathbf{q}=0} \ . \tag{S18}$$

we can recast the expanded eigenfunction-eigenvalue equation for $\mathcal{H}(\mathbf{r}, \mathbf{r}')$ in the form

$$\begin{aligned}
&\left\{1 + \left(-i\nabla + \frac{2e}{\hbar}\mathbf{A}\right)\cdot\nabla_{\mathbf{q}} \right. \\
&\left. + \frac{1}{2}\left[\left(-i\nabla + \frac{2e}{\hbar}\mathbf{A}\right)\cdot\nabla_q\right]^2\right\}\mathcal{H}\,|_{\mathbf{q}=0}\,\psi(\mathbf{r}) \\
&= \mathcal{E}\psi(\mathbf{r}) \ .
\end{aligned} \tag{S19}$$

We consider a magnetic field $\mathbf{B}$ along the $\hat{y}$ axis. In the Landau gauge, $\mathbf{B}$ can be expressed as the curl of the vector potential $\mathbf{A} = \{A_x = B_\perp z, A_y = 0, A_z = 0\}$. Hence Eq. (S19) becomes

$$\begin{aligned}
&\Bigg\{\frac{1}{\tau_\varphi} + D\left[Q_+^2 + Q_3^2\right] J_z^2 + \left[Q_-^2 + Q_3^2\right] J_x^2 \\
&- 2DQ_+ J_z\left(-i\nabla_x + \frac{2eB_\perp}{\hbar} z\right) + 2DQ_- J_x\left(-i\nabla_z\right) \\
&+ D\left(-i\nabla_x + \frac{2eB_\perp}{\hbar} z\right)^2 + D\left(-i\nabla_z\right)^2\Bigg\}\psi(\mathbf{r}) = \mathcal{E}\psi(\mathbf{r}),
\end{aligned} \tag{S20}$$

with $\mathcal{H}(\mathbf{q})$ and its derivatives obtained from Eq.(S13). We now introduce $z_0 = k_x\hbar/2eB$ ($k_x$ is the Cooperon wavevector along the $\hat{x}$ direction) and define the canonical transformation,

$$\begin{aligned}
-i\nabla_z &= \sqrt{\tfrac{2eB_\perp}{\hbar}}\,\tfrac{(a-a^\dagger)}{i\sqrt{2}}\ , \\
z + z_0 &= \tfrac{1}{\sqrt{\frac{2eB_\perp}{\hbar}}}\,\tfrac{(a+a^\dagger)}{\sqrt{2}}\ ,
\end{aligned} \tag{S21}$$

so as to write Eq. (S20) into the number representation,

$$\begin{aligned}
&\Bigg\{\frac{1}{\tau_\varphi} + D\left(Q_+^2 + Q_3^2\right) J_z^2 + \left(Q_-^2 + Q_3^2\right) J_x^2 \\
&- DQ_+ J_z\sqrt{\frac{4eB_\perp}{\hbar}}(a + a^\dagger) - iDQ_- J_x\sqrt{\frac{4eB_\perp}{\hbar}}(a - a^\dagger) \\
&+ D\left(\frac{4eB_\perp}{\hbar}\right)\left(a^\dagger a + \frac{1}{2}\right)\Bigg\}|u\rangle = \mathcal{E}|u\rangle\ ,
\end{aligned} \tag{S22}$$

where $|u\rangle$ is the corresponding eigenket. Equation (S22) maintains the structure of the original Cooperon in spin space (c.f. the corresponding eigenvalue equation for $\mathcal{H}$ in Eq. S13), with $q^2$ being replaced by $\frac{4eB_\perp}{\hbar}\left(a^\dagger a + \frac{1}{2}\right)$, while its components $q_x$ and $q_z$ were replaced by $\sqrt{\frac{4eB_\perp}{\hbar}}(a+a^\dagger)/2$ and $\sqrt{\frac{4eB_\perp}{\hbar}}(a-a^\dagger)/2i$ respectively. To simplify our notation, in what follows we introduce the following effective magnetic fields [1]: $B_\varphi = \hbar/4eD\tau_\varphi$, $B_{SO+} = \hbar Q_+^2/4e$, $B_{SO-} = \hbar Q_-^2/4e$ , $B_{SO3} = \hbar Q_3^2/4e$, $B_{tr} = \hbar/4eD\tau_1$. Note that the solution of Eq. (S22) is obtained as a spinor in the 4-dimensional spin space corresponding to the tensor product of the two spin operators associated with the incident and scattered particle, respectively. In what follow we work on the basis $J, J_z$ of the total angular momentum $J = 0$ and $J = 1$ and

their corresponding z-components $J_z = 0$ and $J_z = 1, 0 - 1$.

The *singlet* $J = 0,\ J_z = 0$ solution is immediately factored, as it is diagonal both in the spin and Landau level spaces. The $n$-th singlet Landau eingenvalue is

$$\mathcal{E}_0 = \frac{4DeB_\perp}{\hbar}\left(n + \frac{1}{2} + \frac{B_\varphi}{B_\perp}\right) , \tag{S23}$$

or

$$\tilde{\mathcal{E}}_{n,0} = \frac{\mathcal{E}_0}{\frac{4DeB_\perp}{\hbar}} = \left(n + \frac{1}{2} + \frac{B_\varphi}{B_\perp}\right) , \tag{S24}$$

The *triplet* solutions can be obtained from Eq. (S22) (with $4eDB_\perp/\hbar$ factored out) written as a $3 \times 3$ matrix in the basis of $J = 1,\ J_z = 1, 0, -1$ via

$$\begin{vmatrix} \begin{matrix}\frac{B_\varphi}{B_\perp} + \frac{B_{SO+}}{B_\perp} + \frac{B_{SO-}+3B_{SO3}}{2B_\perp} \\ +a^\dagger a + \frac{1}{2} - \sqrt{\frac{B_{SO+}}{B_\perp}}(a + a^\dagger) - \tilde{\mathcal{E}}\end{matrix} & -i\sqrt{\frac{B_{SO-}}{2B_\perp}}(a - a^\dagger) & \frac{B_{SO-}+B_{SO3}}{2B_\perp} \\ -i\sqrt{\frac{B_{SO-}}{2B_\perp}}(a - a^\dagger) & \frac{B_\varphi}{B_\perp} + \frac{B_{SO-}+B_{SO3}}{B} + a^\dagger a + \frac{1}{2} - \tilde{\mathcal{E}} & -i\sqrt{\frac{B_{SO-}}{2B_\perp}}(a - a^\dagger) \\ \frac{B_{SO-}+B_{SO3}}{2B_\perp} & -i\sqrt{\frac{B_{SO-}}{2B_\perp}}(a - a^\dagger) & \begin{matrix}\frac{B_\varphi}{B_\perp} + \frac{B_{SO+}}{B_\perp} + \frac{B_{SO-}+3B_{SO3}}{2B_\perp} \\ +a^\dagger a + \frac{1}{2} + \sqrt{\frac{B_{SO+}}{B_\perp}}(a + a^\dagger) - \tilde{\mathcal{E}}\end{matrix} \end{vmatrix} = 0 , \tag{S25}$$

where $\tilde{\mathcal{E}} = \mathcal{E}/(4DeB_\perp/\hbar)$.

In the limit where the two linear SOI constants are almost equal, $B_{SO-} \ll B_{SO+}$ and $B_{SO3} \ll B_{SO+}$, we can justifiably drop all off-diagonal terms proportional with $B_{SO-}$ or $B_{SO-} + B_{SO3}$ in Eq. (S25). This regime corresponds to a decreased coupling between the triplet modes within the same Landau level as the scattering processes do not involve spin flip. The original orientation of the incident particle is preserved as the electron population becomes polarized by the effective field $B_{SO+}$ along the $\hat{z}$ axis. As a further simplification, we perform another canonical transformations on the operators $a, a^\dagger$ in order to incorporate the additional translation proportional to $Q_+$,

$$\begin{aligned} -i\nabla_z &= \sqrt{\tfrac{2eB_\perp}{\hbar}}\,\tfrac{(a-a^\dagger)}{i\sqrt{2}} , \\ z + z_0 \mp \frac{\hbar Q_+}{2eB_\perp} &= \tfrac{1}{\sqrt{\frac{2eB_\perp}{\hbar}}}\,\tfrac{(a+a^\dagger)}{\sqrt{2}} , \end{aligned} \tag{S26}$$

where $\mp$ correspond to $J_z = \pm 1$, respectively.

The diagonalization of Eq. (S25) can be done separately for each spin mode straightfor-

wardly as the determinant is diagonal. We find

$$\tilde{\mathcal{E}}_{n,1} = \tilde{\mathcal{E}}_{n,2} = n + \tfrac{1}{2} + \tfrac{B_\varphi}{B_\perp} + \tfrac{B_{SO-}+3B_{SO3}}{2B_\perp}, \tag{S27}$$

$$\tilde{\mathcal{E}}_{n,3} = n + \tfrac{1}{2} + \tfrac{B_\varphi}{B_\perp} + \tfrac{B_{SO-}+B_{SO3}}{B_\perp}\ , \tag{S28}$$

where for convenience we have indexed the eigenvalues as $\tilde{\mathcal{E}}_{n,1}$, $i = 1, 2, 3$ corresponding to the triplets with $J_z = 1, -1, 0$.

To calculate the corrections to the conductivity associated with Landau level diagonal modes we have to replace the integral over $\mathbf{q}$ in Eq. S3 by a discrete sum over the occupied Landau levels, i.e.,

$$\frac{1}{2\pi}\int_0^{q_{max}} q dq \to \frac{1}{4\pi}\frac{4eB_\perp}{\hbar}\sum_{n=0}^{n_m}\ , \tag{S29}$$

where we have used $q^2 = \frac{4eB_\perp}{\hbar}\left(n+\frac{1}{2}\right)$ ($q^2$ is quantized) thus leading to $2qdq = \frac{4eB_\perp}{\hbar}\Delta n = \frac{4eB_\perp}{\hbar}$, since $\Delta n = 1$ (the minimum variation in the sum over $n$). $n_m$ is given from the condition $q^2_{max} = \frac{4eB_\perp}{\hbar} n_m = (D\tau_1)^{-1}$, which is the maximum momentum exchanged allowed given by the transport time in the diffusion approximation. This gives $n_m = \hbar/(4eB_\perp D\tau_1) = B_{tr}/B_\perp$. Following the angular integration of Eq. (S10), by using Eqs. (S24) and (S27), we obtain

$$\begin{aligned}\Delta\sigma \sim \sum_{n=0}^{n_m}\sum_{i=0,3}\tfrac{1}{\tilde{\mathcal{E}}_{n,i}} = \textstyle\sum_{n=0}^{n_m}\Bigg\{&\frac{2}{n+\frac{1}{2}+\frac{B_\varphi}{B_\perp}+\frac{B_{SO-}+3B_{SO3}}{2B_\perp}} + \\ &\frac{1}{n+\frac{1}{2}+\frac{B_\varphi}{B_\perp}+\frac{B_{SO-}+B_{SO3}}{B_\perp}} + \frac{1}{n+\frac{1}{2}+\frac{B_\varphi}{B_\perp}}\Bigg\}\ .\end{aligned} \tag{S30}$$

Since we consider $n_m \gg 1$, we can manipulate the sums over $n$ in the following way. For properly defined $a$'s, the sums in Eq. (S30) have the generic form

$$\begin{aligned}\sum_{n=0}^{n_m}\frac{1}{n+a} &= \sum_{n=0}^{n_m}\frac{1}{n+a} - \sum_{n=1}^{n_m}\frac{1}{n} + \sum_{n=1}^{n_m}\frac{1}{n} \\ &= -\sum_{n=1}^{n_m}\frac{a-1}{n(n+a-1)} + C + \ln n_m \\ &= -\Psi(a) + \ln n_m\ ,\end{aligned} \tag{S31}$$

where we have used the definition of the Euler constant $C$,

$$C = \lim_{n\to\infty} \left( \sum_{k=1}^{n} \frac{1}{k} - \ln n \right) \ , \tag{S32}$$

and of the Digamma function,

$$\Psi(a+1) = -C + \sum_{n=1}^{\infty} \frac{a}{n(n+a)} \ . \tag{S33}$$

*Final formula for the weak localization corrections.* Following the algorithm outlined above, we obtain the corrections to the conductivity as

$$\begin{aligned} \Delta\sigma(B_\perp) = -\frac{e^2}{4\pi^2\hbar} \Bigg[ & \Psi\left(\frac{1}{2} + \frac{B_\varphi}{B_\perp}\right) + 2\ln\frac{B_{\rm tr}}{B_\perp} - 2\Psi\left(\frac{1}{2} + \frac{B_\varphi}{B_\perp} + \frac{B_{SO-} + 3B_{SO3}}{2B_\perp}\right) \\ & -\Psi\left(\frac{1}{2} + \frac{B_\varphi}{B_\perp} + \frac{B_{SO-} + B_{SO3}}{B_\perp}\right)\Bigg] . \end{aligned} \tag{S34}$$

The closed-form formula in Eq. (S34) (same as Eq (5) in the main text) is the main theoretical result of this paper. It plays a crucial role in the two-stage fitting procedure we have used to accurately extract all the SO parameters from our thorough weak (anti) localization measurements. We note that (S34) accounts not only for the linear Rashba and Dresselhaus contributions but also for the cubic Dresselhaus term.

## II. FULL ACCOUNT OF DATA

We account for all data measured on samples I and II in Fig. S1 - S5 in the same order as in Fig. 4 of the main text. The data shown in Fig. S1 - S5 was obtained by measuring first sample I and II, which was done twice within the same cooldown, giving the datasets 1 - 4. Dataset 5 shows data on sample II after a thermal cycle. To test the concept of our method, we took data on another sample with a 9.3 nm thick, asymmetrically doped quantum well (sample III), where no WAL is observed at $\alpha = \beta$. To obtain results, we calculated the value of $B_{\rm SO3}$ with the previously determined values of $\gamma$ and $\tau_3/\tau_1$ and only obtained $\tau_\varphi$ in the first evaluation step and then the value of $B_{SO-}$ as in the other cases. The corresponding data is shown in Fig. S6.

### A. Summary of extracted data

We first summarize the extracted values of the SO parameters $\alpha_0$, $\alpha_1$ and $\gamma$, the scattering time ratio $\tau_3/\tau_1$ and the effective distances $d_T$ and $d_B$ for each sample. The values of $d_T$ and $d_B$ are extracted from fits to the density map over the same range of gate voltages, where the contours of constant density are linear. We note that the value of $d_B$ in measurement #5 & #6 is smaller, because measurement #5 corresponds to a different cooldown and measurement #6 to a different sample and wafer. The epitaxial values of $d_T$ and $d_B$ are 75 nm and 1210 nm. The significantly smaller value of $d_B$ is due to the low temperature grown GaAs buffer layer of 600 nm.

TABLE I. All relevant extracted data for the different samples.

| Measurement # | Sample | $\alpha_0$ [meVÅ] | $\alpha_1$ [eÅ$^2$] | $\gamma$ [eVÅ$^3$] | $\tau_3/\tau_1$ | $d_T$ [nm] | $d_B$ [nm] |
|---|---|---|---|---|---|---|---|
| 1 | 11 nm - I | 1.7±0.6 | 9.3±0.3 | 13.4±1.2 | 0.21 | 107 | 750 |
| 2 | 11 nm - II | 1.3±1.0 | 9.4±0.3 | 12.3±2.0 | 0.24 | 101 | 765 |
| 3 | 11 nm - I | 0.9±0.7 | 9.8±0.2 | 10.2±1.4 | 0.37 | 107 | 750 |
| 4 | 11 nm - II | 0.4±1.3 | 9.9±0.4 | 8.6±2.4 | 0.47 | 101 | 765 |
| 5 | 11 nm - II | 1.6±1.4 | 8.4±0.3 | 12.8±2.7 | 0.23 | 102 | 736 |
| 6 | 9.3 nm - III | 5.5±0.4 | 9.0±0.1 | 15.3±0.7 | 0.16 | 100 | 710 |

The following figures are organized as follows: The density map is shown in panel (a), with the contours indicating the respective value of the density (in multiples of $10^{15}\,\mathrm{m}^{-2}$). The markers correspond to the manually determined symmetry points, the line in the same color corresponds to the expected symmetry points from the extracted SO parameters and the broken blue line corresponds to the expected symmetry points using the average of the extracted SO parameters. Panel (b) shows the contours of constant mobility with its values indicated in m$^2$/Vs. Panel (c) shows the fits to the WAL traces at $\alpha \approx \beta$ for all measured densities. Panel (d) shows the extracted values of $B_{SO3}$, $B_\varphi$, $\tau_3/\tau_1$ and $\tau_\varphi$ for the measured densities. Panel (e) and (f) show the extracted values of $B_{SO-}$ (green markers) and its fit (blue line) for each density, indicated in multiples of $10^{15}\,\mathrm{m}^{-2}$.

*a. Dataset 1.*

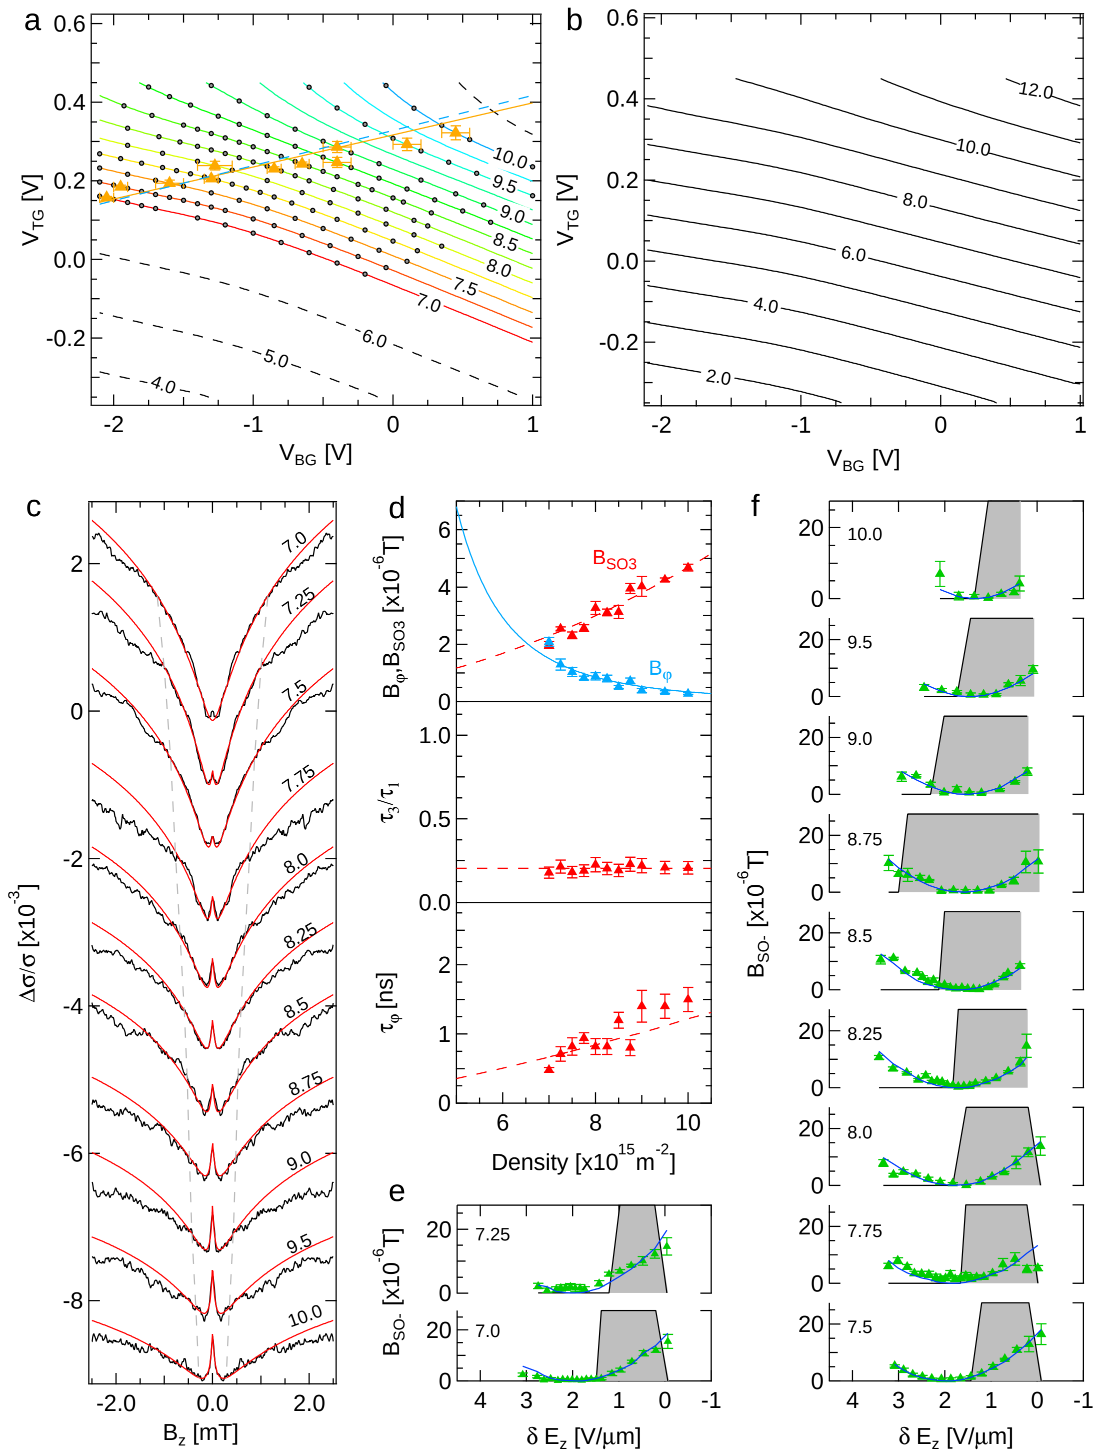


FIG. S1. First measurement on sample I. Gate configurations were measured not in a particular order and their spacing in back gate voltage is not equidistant, because at this stage the method how to aquire data most reliably, was still in development.

*b. Dataset 2.*

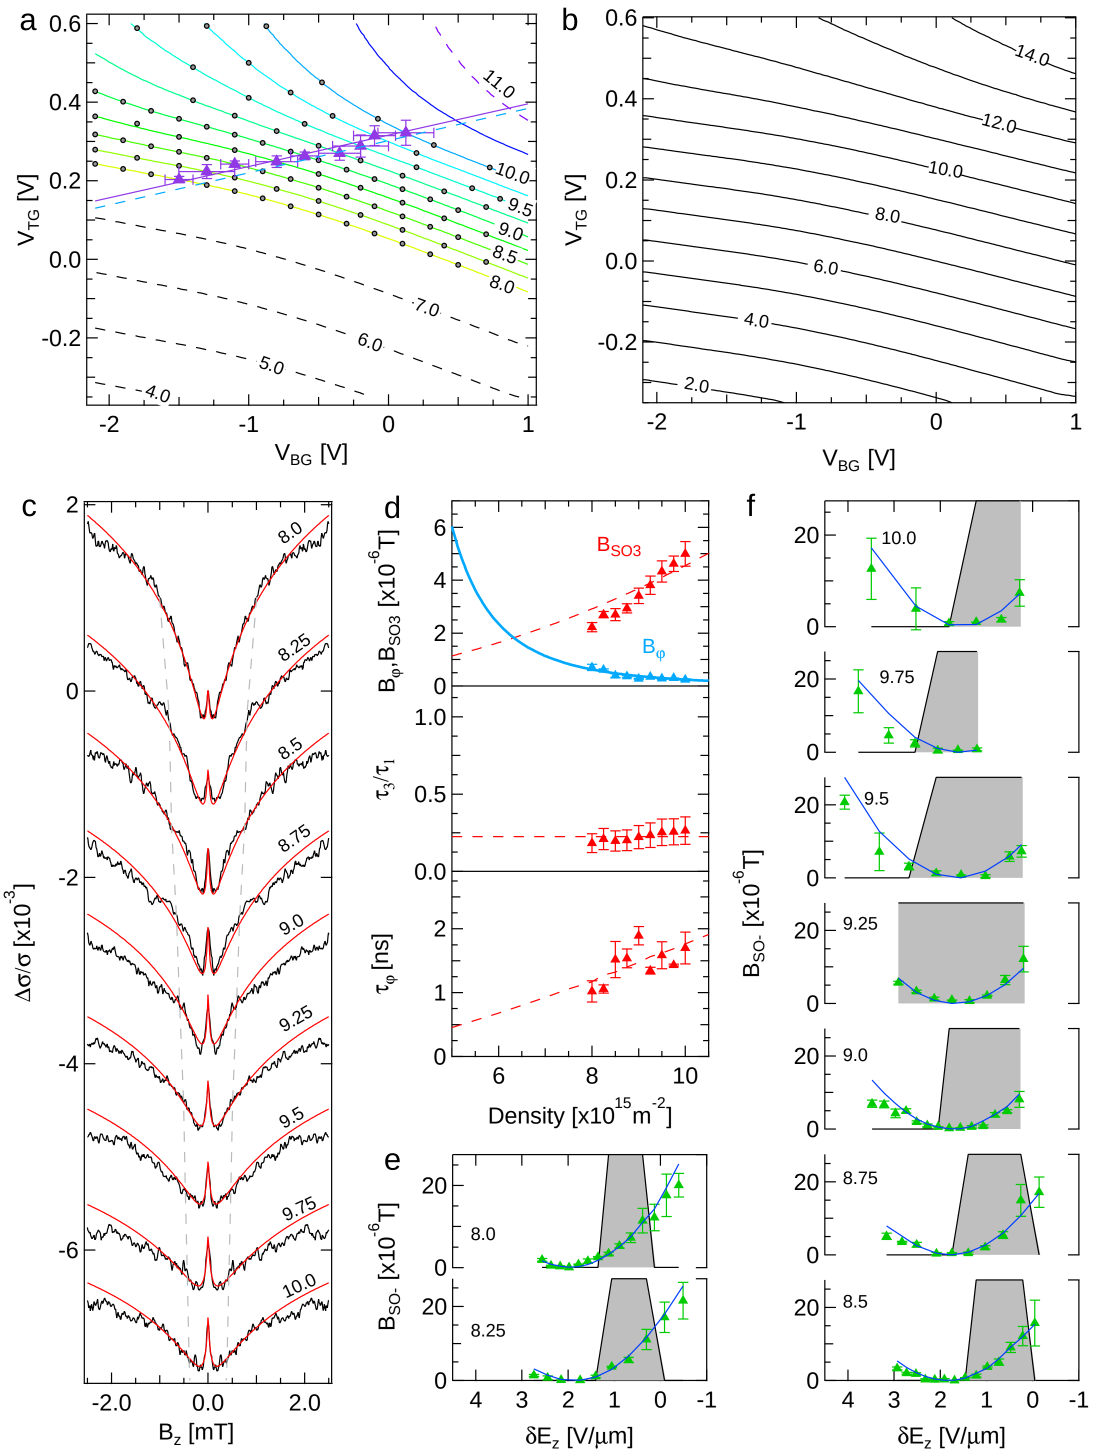


FIG. S2. First measurement on sample II. The mobility is slightly higher as in sample I. Data are taken sequentially and back gate voltage spacing is chosen to be the same for each density.

*c. Dataset 3.*

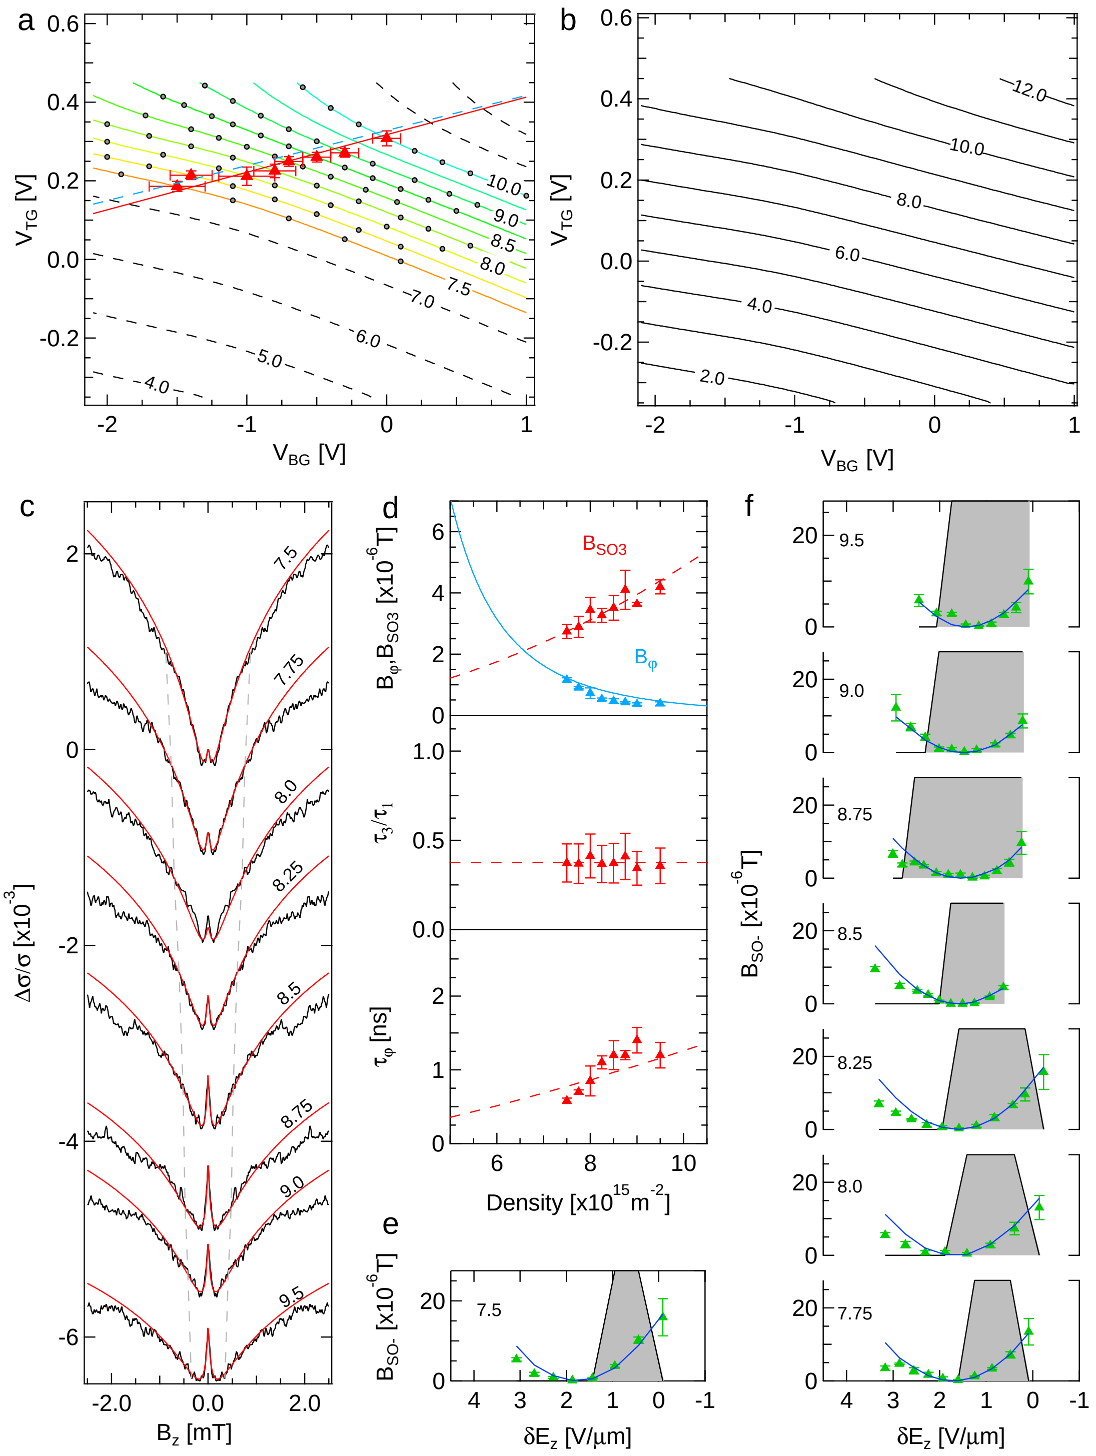


FIG. S3. Second measurement on sample I, the data are aquired here as in the case of dataset 2. The spacing between the gate configurations is the same for each density.

*d. Dataset 4.*

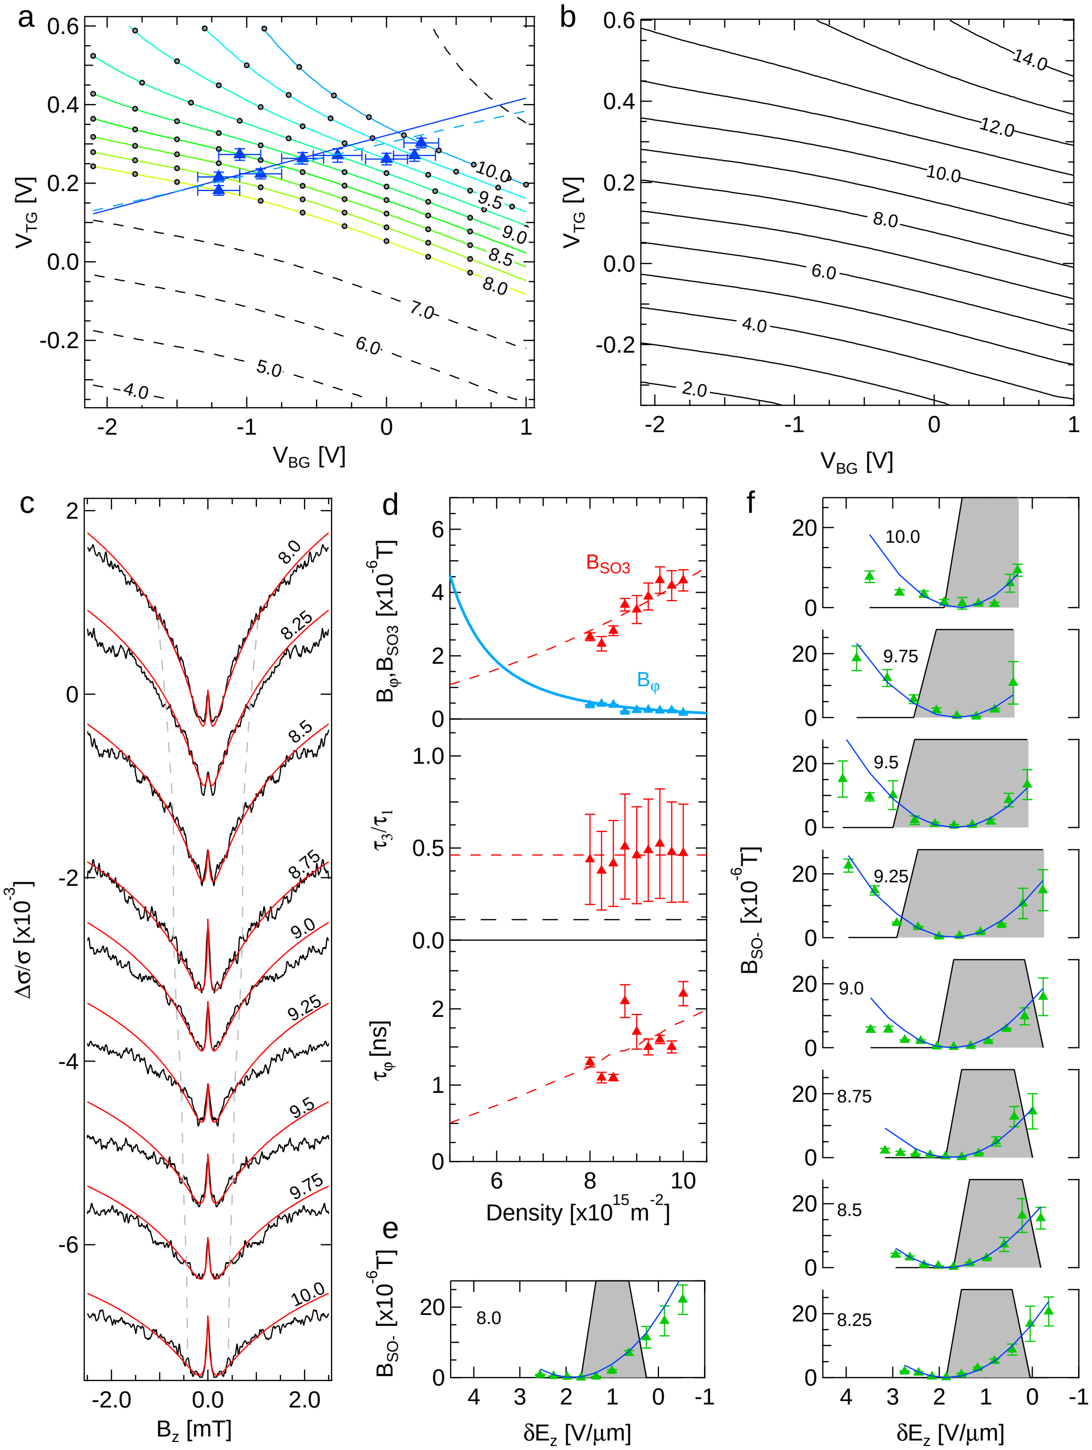


FIG. S4. Second measurement on sample II, as in the previous measurements. Panel (d) middle: The error bars on $\tau_3/\tau_1$ are so large because of the low value of $\gamma \sim 8.6$ eVÅ$^3$. The black dashed line corresponds to the theoretical minimum of $\tau_3/\tau_1$.

*e. Dataset 5.*

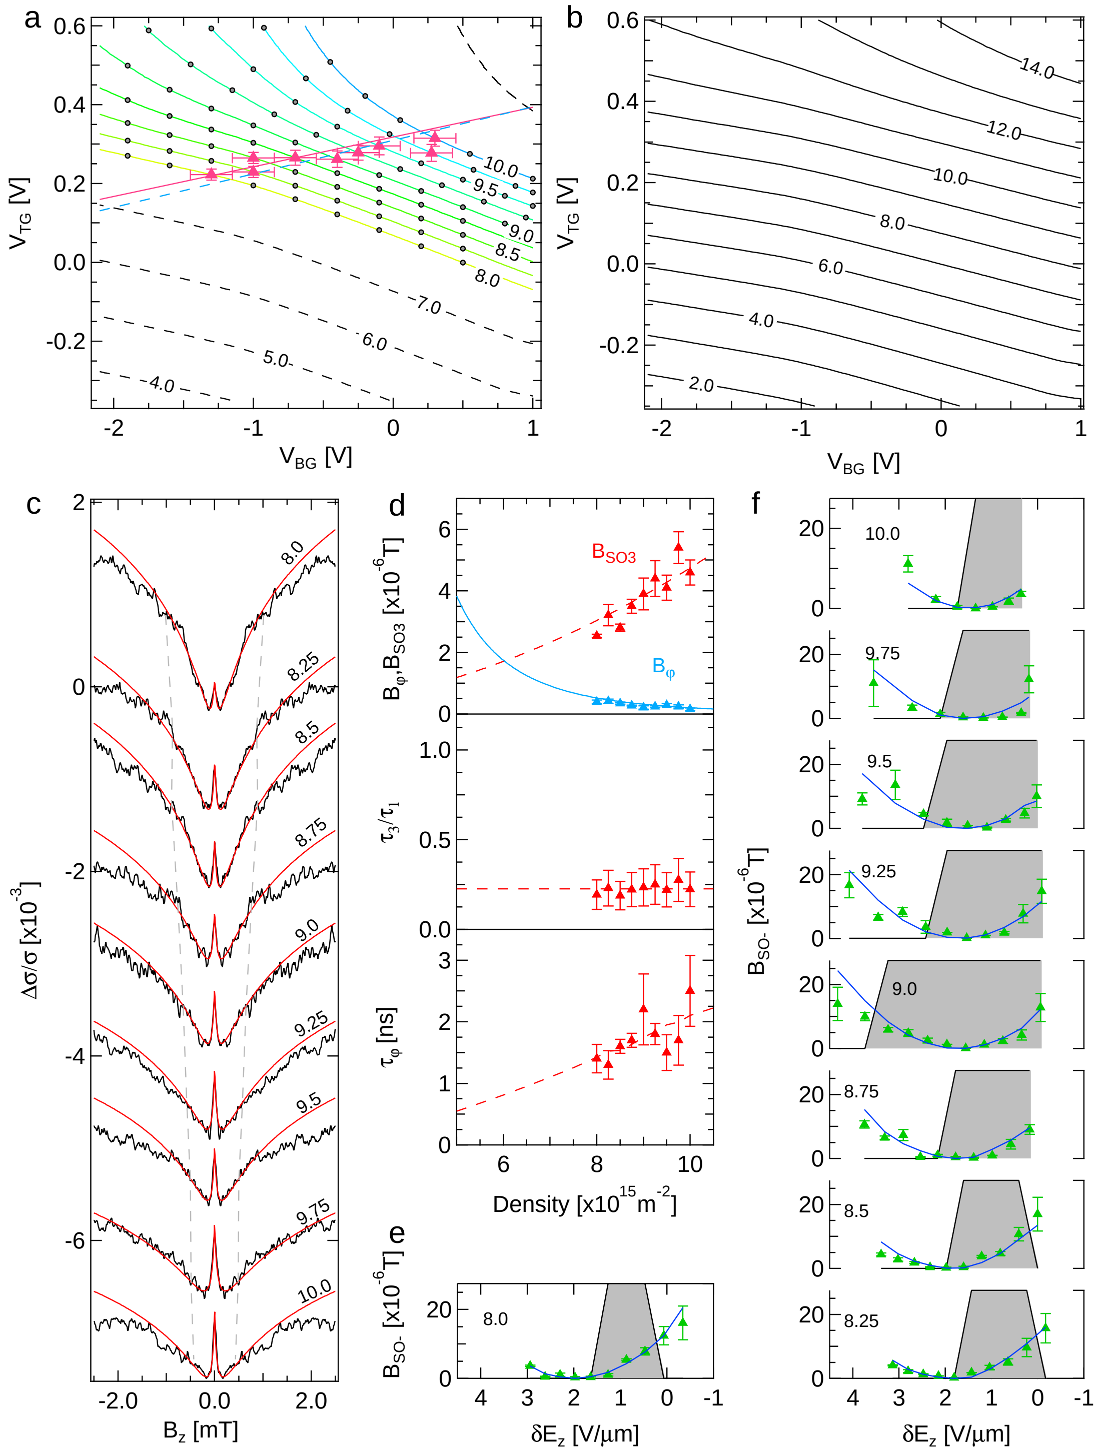


FIG. S5. Third measurement on sample II in another cooldown.

*f. Dataset 6.* Data from another wafer, which is doped asymmetrically and has a 9.3 nm thick QW. The densities are much lower in this wafer resulting in a full suppression of WAL at $\alpha \approx \beta$. The extracted SO values are within the range of the expected values for this wafer, except the value of $\gamma$, which is larger than expected and we do not understand it fully at this point.

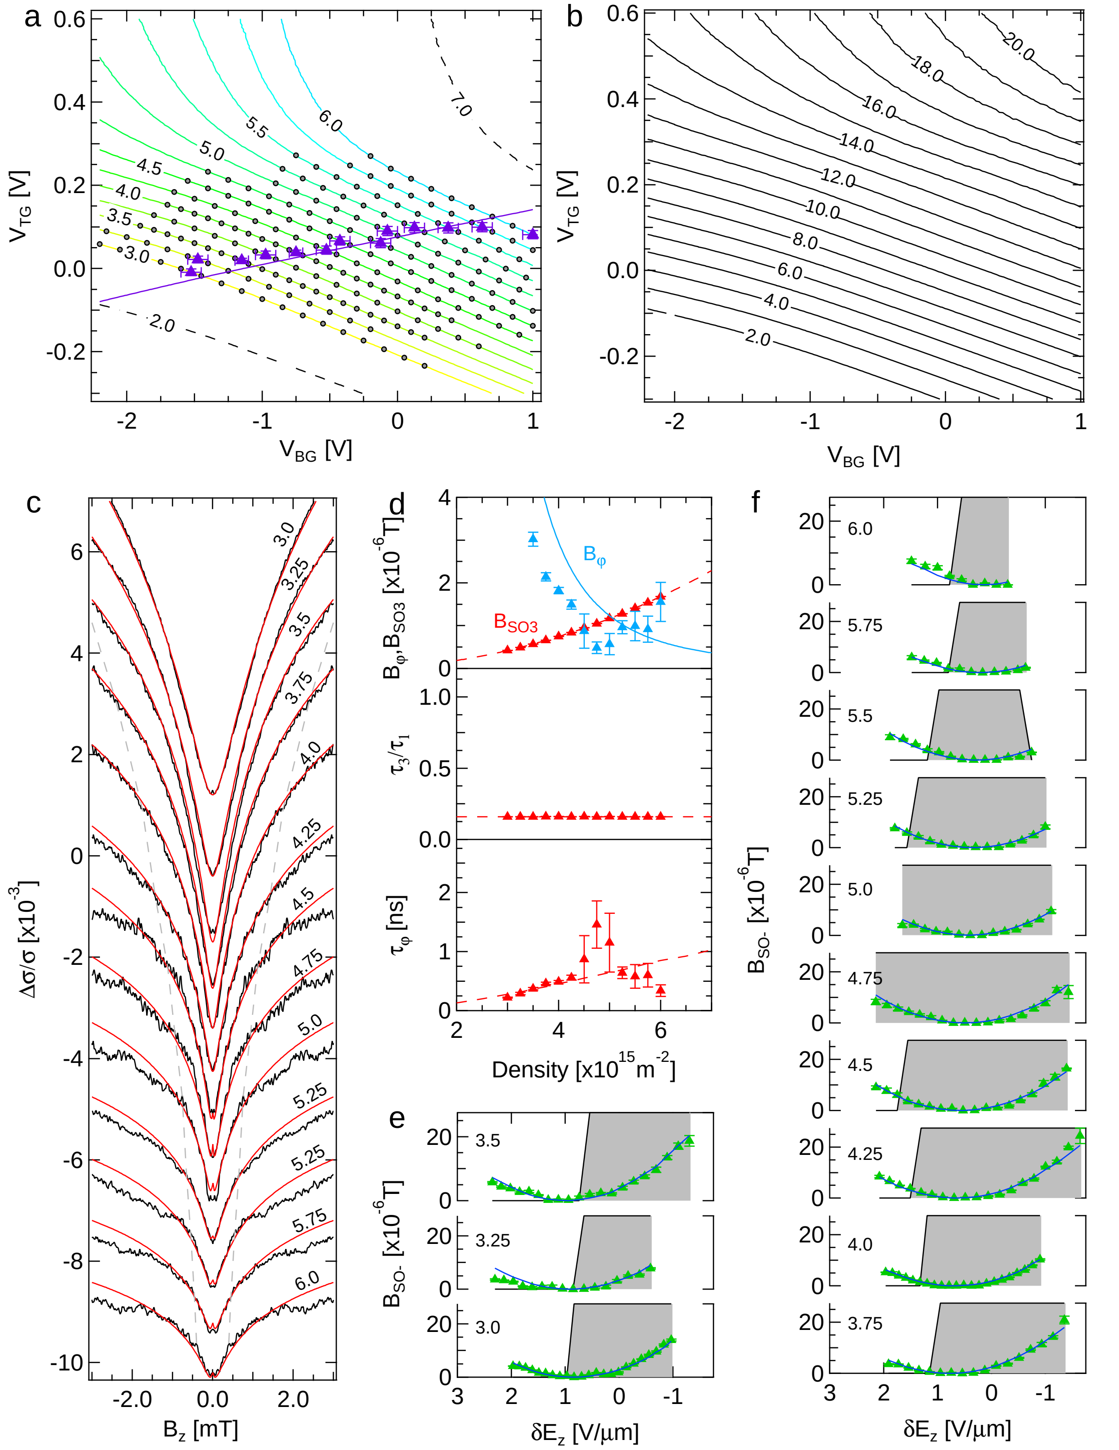


FIG. S6. First measurement on sample III (9.3 nm quantum well, asymmetrically doped).

## III. DETAILS ON EVALUATING $B_{SO-}$ AND $B_{SO3}$

### A. Symmetry point determination and value of $B_{SO3}$

Here, we show how the value of $B_{SO3}$ and the position of the symmetry point are determined from the WAL traces. The data presented is from measurement 3 at a density of $8.25 \times 10^{15}\,\mathrm{m}^{-2}$. Figure S7(a) shows the measured magnetoconductance traces along a contour of constant density. We can clearly see how the WAL peak gets smaller with more positive gate voltage and then starts to increase again. As described in the main text we fit the expression for the quantum corrections and extract an *effective* SO value called $B^{*}_{SO3}$ for each gate configuration, which will have a minimum around $\alpha \approx \beta$, see Fig. S7(b), as the difference of between $\alpha$ and $\beta$ should be very small and only the cubic term remains. To obtain a value of $B_{SO3}$, we perform fits to the WAL trace at the minimum and $\pm 1$ trace from it, using Eq. (S34), where $B_{\mathrm{SO}-}$ is set to zero, see Fig. S7(c)-(e). The final value for $B_{SO3}$ and $\tau_\varphi$ is obtained by taking the average of the three respective values.

### B. Validity of the theory

With the known values of $B_{SO3}$ and $\tau_\varphi$ the value of $B_{SO-}$ can be extracted from each WAL trace. Here we show all measured magnetoconductivity traces with their respective fits to the data of dataset 3. We can see that these fits give in general very good agreement within the allowed fit range, given by $B_{\mathrm{SO}-}, B_{\mathrm{SO3}} \ll B_{\mathrm{tr}}$ the gray dashed line in each graph corresponds to $B_\perp = 0.5 B_{\mathrm{tr}}$. For WAL traces measured at more positive back gate voltage, the fit no longer captures the full WAL trace, especially at low densities ($n = 7.5 - 8.25 \times 10^{15}\mathrm{m}^{-2}$), the extracted values of $B_{SO-}$ from these curves are then disregarded. The respective traces are colored in gray.

The exclusion of the results from the fits to these traces also serves as a validity check of the new theory. Equation (S34) is obtained in the limit of $B_{\mathrm{SO}-} \ll B_{SO+}$. Using the expressions for $B_{\mathrm{SO}\pm}$ we can rewrite the condition and obtain in terms of $\alpha$ and $\beta$:

$$r \equiv \left| \frac{\alpha - \beta}{\alpha + \beta} \right| \ll 1, \tag{S35}$$

which sets the range of the applicability of Eq. (S34) of the main text. By setting $r \sim 0.4$,

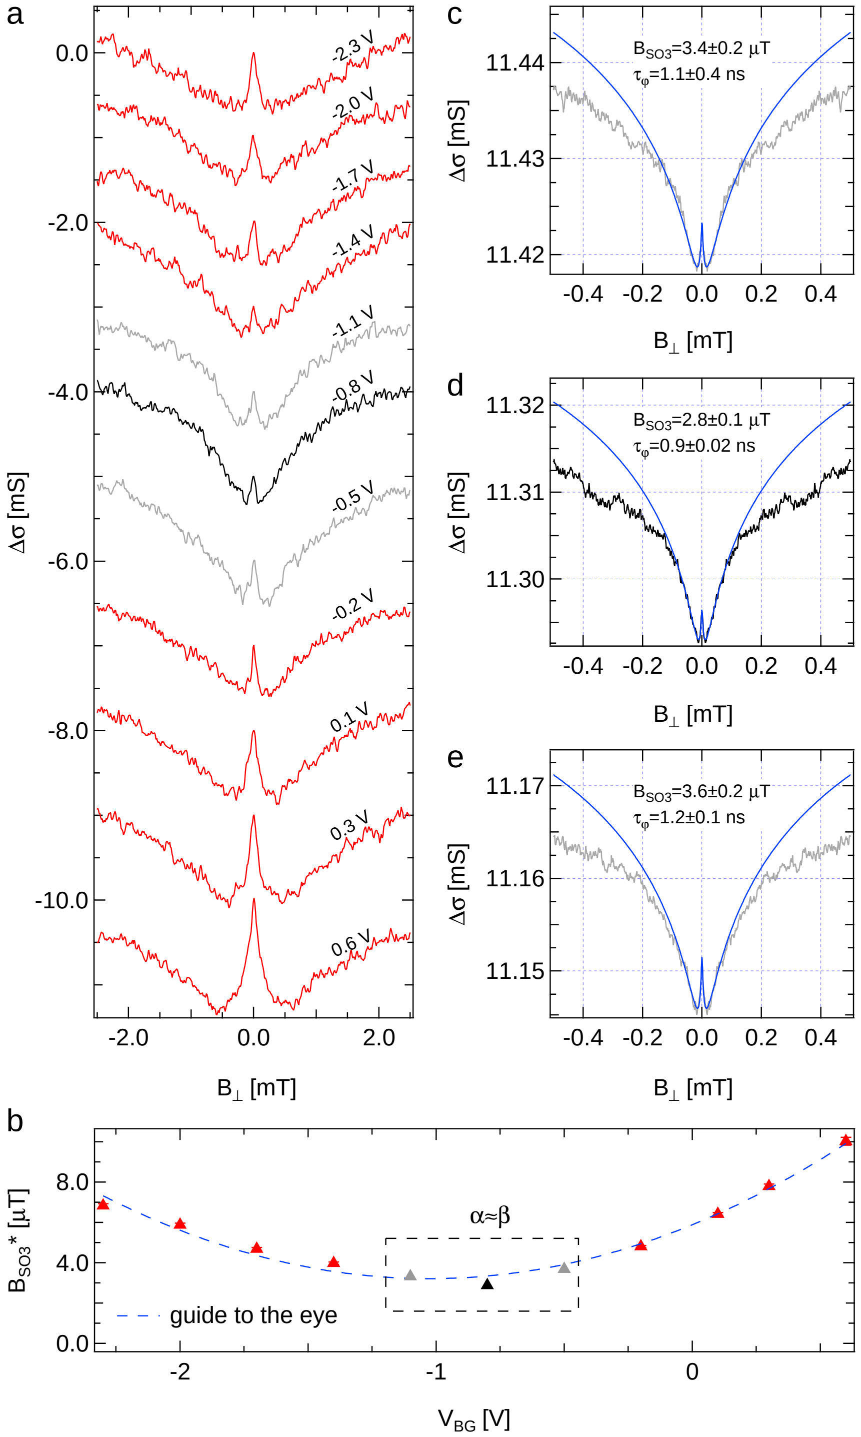


FIG. S7. Determination of $\alpha \approx \beta$ for measurement 3. Panel (a) shows the WAL traces with their gate voltage indicated. In (b) the obtained values of $B^{*}_{SO3}$ are shown as a function of back gate, showing a minimum at around -0.7 V. The blue dashed curve is a guide to the eye. Panels (c) to (e) show fits to the corresponding WAL traces around the minimum. The black trace is where the WAL peak is almost suppressed. This is the point, where $\alpha \approx \beta$.

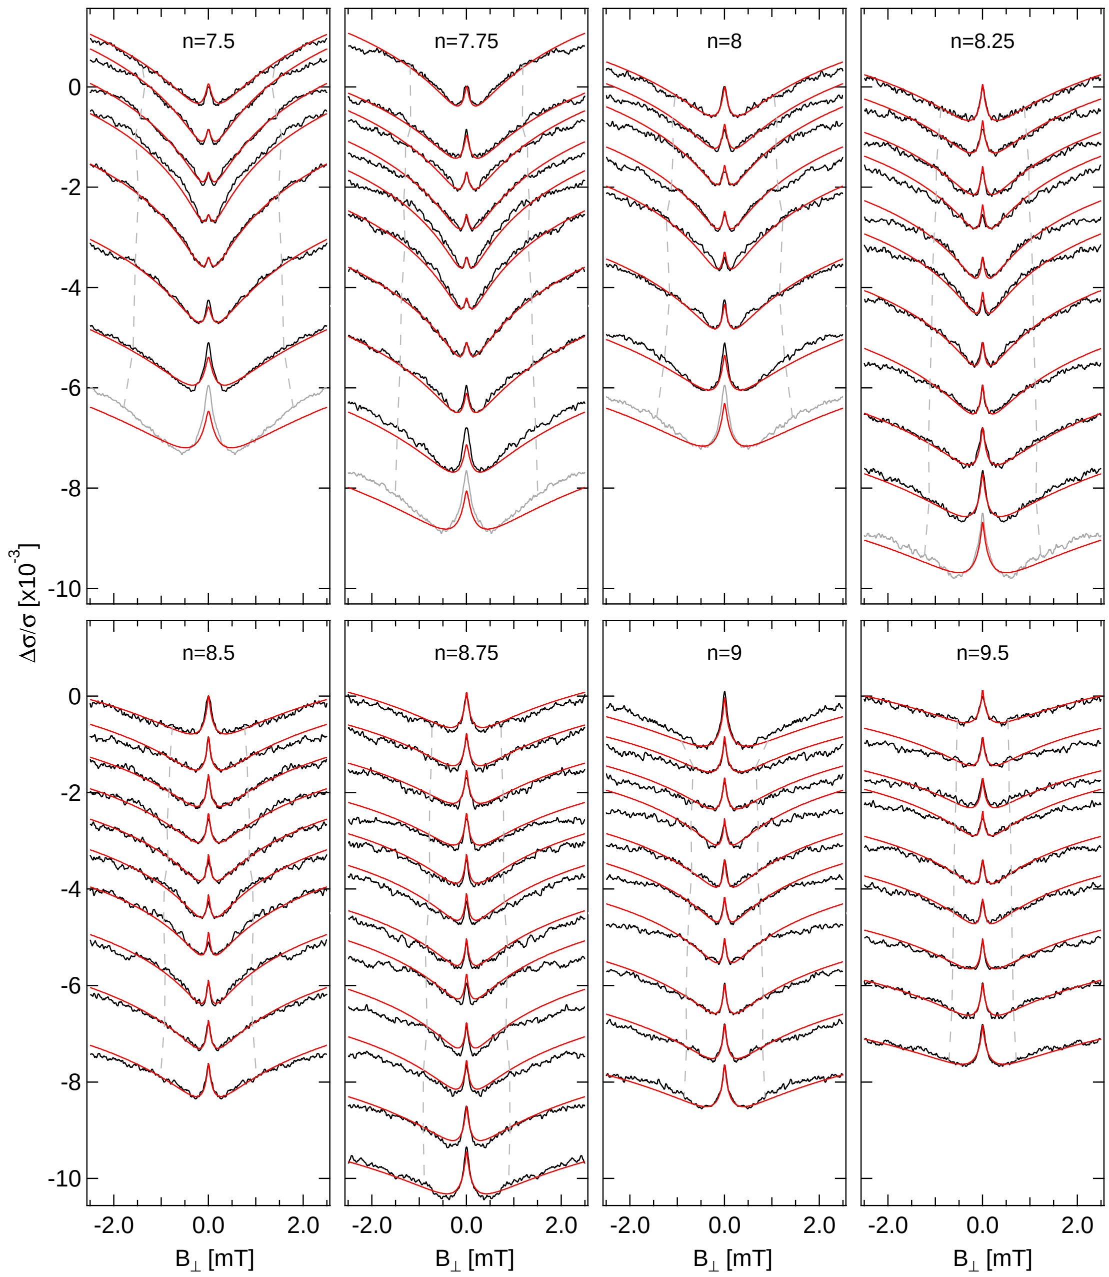


FIG. S8. Fits to WAL traces with only $B_{SO-}$ as a fit parameter for dataset 3. Each panel corresponds to one density and the magnetoconductivity traces are organized from top to bottom with increasing backgate voltage from negative to positive. The gray dashed line sets an upper bound to the allowed fit range for each individual trace, given by $B_\perp = 0.5B_{\rm tr}$

a validity range can be defined in terms of top and back gate voltages. This range has to be compared with the gate configurations measured and agrees well with the manually excluded

gate configurations.


[1] S. Iordanskii, Y. Lyanda-Geller, and G. Pikus, *Weak Localization in Quantum Wells with Spin-Orbit Interaction,* JETP Letters **60**, 199 (1994).

[2] W. Knap, C. Skierbiszewski, A. Zduniak, E. Litwin-Staszewska, D. Bertho, F. Kobbi, J. L. Robert, G. E. Pikus, F. G. Pikus, S. V. Iordanskii, V. Mosser, K. Zekentes, and Y. B. Lyanda-Geller, *Weak antilocalization and spin precession in quantum wells,* Physical Review B **53**, 3912 (1996).

[3] D. C. Marinescu, *Cubic Dresselhaus interaction parameter from quantum corrections to the conductivity in the presence of an in-plane magnetic field,* Physical Review B **96**, 115109 (2017).

[4] L. Gor'kov, A. Larkin, and D. Khmel'nitskii, *Particle conductivity in a two-dimensional random potential,* JETP Letters **30**, 228 (1979).

[5] S. Hikami, A. I. Larkin, and Y. Nagaoka, *Spin-Orbit Interaction and Magnetoresistance in the Two Dimensional Random System,* Progress of Theoretical Physics **63**, 707 (1980).

[6] F. G. Pikus and G. E. Pikus, *Conduction-band spin splitting and negative magnetoresistance in A3B5 heterostructures,* Physical Review B **51**, 16928 (1995).

[7] B. L. Al'tshuler, A. G. Aronov, A. I. Larkin, and D. E. Khmel'nitskii, *Anomalous magnetoresistance in semiconductors,* Journal of Experimental and Theoretical Physics **54**, 411 (1981).
